# Supplementary material for: Video-MMMU: Evaluating Knowledge Acquisition from Multi-Discipline Professional Videos
Source: arXiv:2501.13826 source file (2025-01-23)
Supplement: Supplementary file 1 [file 8.Appendix.tex]

\appendix

\vspace{10pt} % Adjust vertical space between rows

\begin{subfigure}[b]{0.48\textwidth}
    \centering
    \includegraphics[width=\textwidth]{audio_track_new.pdf}
    \caption{Comparison of Early Failure Rate (the percentage of Right-to-Wrong questions that also failed in their corresponding Perception or Comprehension question).}
    \label{fig:figure6}
\end{subfigure}
\hfill
\begin{subfigure}[b]{0.48\textwidth}
    \centering
    \includegraphics[width=\textwidth]{error_piechar1113.pdf}
    \caption{Comparison of performance before and after adding audio transcripts.}
    \label{fig:audio}
\end{subfigure}

\section{Performance by Discipline}

\begin{table*}[t]
\tabstyle{4pt}
\centering
\makebox[\textwidth][c]{
    \begin{tabular}{lcccccccccc}
    \toprule
\textbf{Model} & \textbf{Params} & \textbf{Frames} & \textbf{Overall} & \textbf{Art} & \textbf{Business} & \textbf{Science} & \textbf{Medicine} & \textbf{Humanities} & \textbf{Engineering} \\
\midrule
\textbf{Random Choice} & -- & -- & 12.17 & 14.81 & 10.83 & 12.75 & 15.87 & 15.00 & 14.28 &  \\
\textbf{Human Expert} & -- & -- & 83.95 & 94.44 & 91.45 & 83.33 &78.43 & 83.83 & 79.80  \\
\midrule
\rowcolor{blue!20} \multicolumn{10}{l}{\textbf{Proprietary LMMs}} \\
\midrule

\textbf{Gemini-Pro-v1.5} & -- & -- & 55.20 & \textbf{74.07} & 53.90 & 47.92 & 41.67 & 60.00 & 52.38 &  \\
\addlinespace[1mm]
\midrule
\addlinespace[1mm]
\textbf{Claude-3-Opus} & -- & -- & 50.44 & 56.79 & 50.36 & 41.67  & 40.00 & 60.83 & 57.14 &  \\
\textbf{Claude-3.5-Sonnet} & -- & -- & 62.79 & 64.87 & 63.79 & 55.56  & \textbf{60.00} & 72.50  & 57.14 &  \\
\addlinespace[1mm]
\midrule
\addlinespace[1mm]

\textbf{GPT4o-mini} &-- & 50 & 53.09 & 37.04 & 56.03 & 50.69 & 35.00 & 73.33 & 45.62 &  \\
\textbf{GPT4o} & -- & 50 & \textbf{66.49} & 63.49 & \textbf{68.96} & \textbf{57.86} & 51.33 & \textbf{84.67} & 57.14 &  \\

\midrule
\rowcolor{blue!10} \multicolumn{10}{l}{\textbf{Open-source LMMs}} \\
\midrule

\textbf{VILA1.5} & 8B & 32 & 36.69 & 45.68 & 30.50 & 36.81 & 33.33 & 41.67 & 23.81 &  \\
\textbf{VILA1.5} & 40B & 32 & 47.44 & 56.79 & 36.17 & 43.06 & 40.00 & 61.67 & 57.81 &  \\

\addlinespace[1mm]
\midrule
\addlinespace[1mm]

\textbf{LongVA} & 7B & 128 & 39.15 & 43.21 & 36.17 & 38.89 & 31.67 & 46.67 & 23.81 &  \\

\addlinespace[1mm]
\midrule
\addlinespace[1mm]

\textbf{Qwen2-VL} & 7B & 64 & 47.62 & 59.26 & 43.26 & 37.50 & 34.59 & 65.83 & 33.33 &  \\

\addlinespace[1mm]
\midrule
\addlinespace[1mm]
\textbf{InternVL2} & 2B & 32 & 29.10 & 32.77 & 27.66 & 31.25 & 35.00  & 24.17 & 23.81 &  \\
\textbf{InternVL2} & 8B & 32 & 50.79 & 59.26 & 50.35 & 50.00 & 31.67  & 56.67 & 47.62 &  \\

\addlinespace[1mm]
\midrule
\addlinespace[1mm]

\textbf{LLaVA-OneVision} & 0.5B & 32 & 20.11 & 8.64 & 18.44 & 21.53 & 23.33 & 27.50 & 14.29 &  \\
\textbf{LLaVA-OneVision} & 7B & 32 & 49.23 & 56.79 & 53.90 & 39.58 & 41.67 & 55.00 & 42.86 &  \\
\textbf{LLaVA-OneVision} & 72B & 32 & 64.87 & 70.37 & \textbf{67.38} & \textbf{55.56} & \textbf{48.33} & 73.33 & 57.14 &  \\
% \textbf{LLaVA-OneVision} & 7B & 8 & 46.21 & 50.44 & 45.66 & 37.5 & 42.70 & 51.38 & 34.21 \\

\addlinespace[1mm]
\midrule
\addlinespace[1mm]

\textbf{LLaVA-Video} & 7B & 64 & 52.38 & 65.43 & 47.52 & 42.36 & 38.33 & 68.33 & 52.38 &  \\
\textbf{LLaVA-Video} & 72B & 64 & \textbf{64.55} & \textbf{77.78} & 65.96  & 47.92 & \textbf{48.33}  & \textbf{90.00} & \textbf{76.19}  \\
% \textbf{LLaVA-Video} & 7B & 8 & \textbf{48.85} & 55.56 & 52.48 & 40.28 & 30.75 & 65.00 & 47.61 &  \\

\bottomrule
    \end{tabular}
}
\captionsetup{justification=centering}
\caption{Video-MMMU Evaluation Results by Discipline.}
\label{tab:domainresult}
\end{table*}
